# Supplementary material for: How nanoporous silicon-polypyrrole hybrids flex their muscles in aqueous electrolytes: In operando high-resolution x-ray diffraction and electron tomography-based micromechanical computer simulations
Source: arXiv:2211.15496 ancillary file (2022-11-28)
Supplement: Supplementary file 1 [file Supplementary_Materials-How_nanoporous_silicon-polypyrrole_hybrids_flex_their_muscles_in_aqueous_electrolytes.pdf]

# **Supporting Information - How Nanoporous Silicon-Polypyrrole Hybrids Flex Their Muscles in Aqueous Electrolytes: In Operando High-Resolution X-Ray Diffraction and Electron Tomography-Based Micromechanical Computer Simulations**

Manuel Brinker,<sup>1,2,3,\*</sup> Marc Thelen,<sup>1,2,3</sup> Manfred May,<sup>1,2,3</sup>  
Dagmar Rings,<sup>4</sup> Tobias Krekeler,<sup>5</sup> Pirmin Lakner,<sup>6,7</sup> Thomas F.  
Keller,<sup>6,7</sup> Florian Bertram,<sup>8</sup> Norbert Huber,<sup>9</sup> and Patrick Huber<sup>1,7,3,†</sup>

<sup>1</sup>*Hamburg University of Technology, Institute for Materials and X-Ray Physics,  
Denickestr. 10, 21073 Hamburg, Germany*

<sup>2</sup>*Center for X-Ray and Nano Science CXNS,  
Deutsches Elektronen-Synchrotron DESY,  
Notkestr. 85, 22607 Hamburg, Germany*

<sup>3</sup>*Center for Hybrid Nanostructures CHyN, Hamburg University,  
Luruper Chaussee 149, 22607 Hamburg, Germany*

<sup>4</sup>*Institute of Materials Physics and Technology,  
Hamburg University of Technology, 21073 Hamburg, Germany*

<sup>5</sup>*Electron Microscopy Unit BEEM, Hamburg University of Technology, 21073 Hamburg, Germany*

<sup>6</sup>*Physics Department, University of Hamburg, 22607 Hamburg, Germany*

<sup>7</sup>*Center for X-ray and Nano Science CXNS,  
Deutsches Elektronen-Synchrotron DESY,  
Notkestr. 85, 22607 Hamburg, Germany*

<sup>8</sup>*Deutsches Elektronen-Synchrotron DESY,  
Notkestr. 85, 22607 Hamburg, Germany*

<sup>9</sup>*Institute of Materials Research, Materials Mechanics,  
Helmholtz-Zentrum Hereon, 21502 Geesthacht, Germany*

## I. ELECTROPOLYMERISATION OF POLYPYRROLE IN POROUS SILICON

The potential evolution during the electropolymerisation of polypyrrole in porous silicon is shown in Figure S2. Firstly, the potential increases from its open circuit potential of approximately 0.1 V to a plateau of 0.65 V within 2000 s. This initial increase in the potential is associated with a starting nucleation of the pyrrole monomers at the bottom of the pores and an ensuing oxidation of the porous silicon pore walls[1]. The subsequent potential plateau at 0.65 V which lasts from 2000 to 7600 s thereby signals the continued growth of the polymer inside the pore space. The following increase of the potential to 0.83 V marks the gradual filling of the pores. At this point, the applied current is switched off. A continuing applied current would lead to a polymerization in the form of a film[1]. Hence, the current is switched off to prohibit the coverage of the sample by bulk polymer. Such a bulk coverage could lead to a distortion of the actuation characteristics of the polypyrrole filled pores. In order to determine the filling degree of the pores the change in mass  $\Delta m$  is gravimetrically determined. The mass of the sample changes by  $\Delta m = 0.009$  g through the polymerization. Hence, considering the volume of the np-Si layer and its porosity  $\Phi$ , the polypyrrole inside the pores has a density of  $\rho_{\text{PPy}} = 1 \text{ gcm}^{-3}$ . A bulk polypyrrole film, synthesized under comparable conditions possesses a density of  $1.5 \text{ gcm}^{-3}$ , which would indicate a reasonable filling degree of 66 %. This would mark more a lower boundary of filling since it has been reported that the polymer density decreases inside porous silicon[1].

---

\* manuel.brinker@tuhh.de

† patrick.huber@tuhh.de

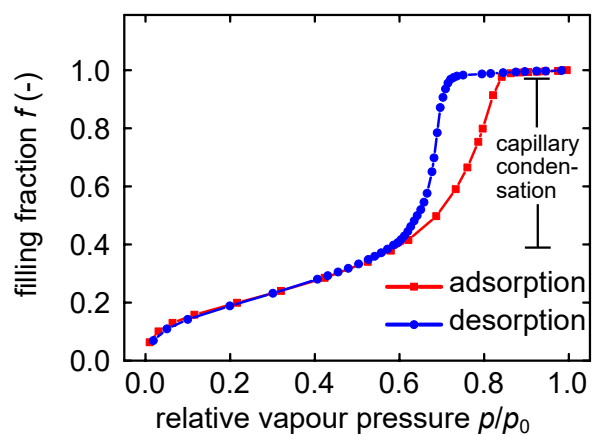

FIG. S1. **Nitrogen sorption isotherm of porous silicon.** Nitrogen sorption isotherm at  $T = 77$  K recorded for the porous silicon layer utilized in this study. Volume filling fraction  $f$  is shown versus the relative vapor pressure  $p/p_0$ .

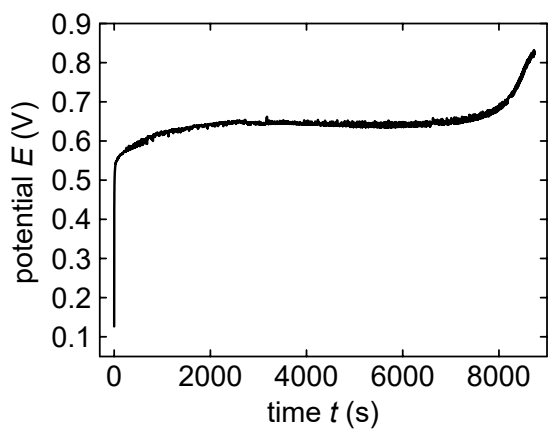

FIG. S2. **Electrochemical polymerisation of polypyrrole in porous silicon.** Time Evolution of potential  $E$  during the electropolymerisation of pyrrole in porous silicon.

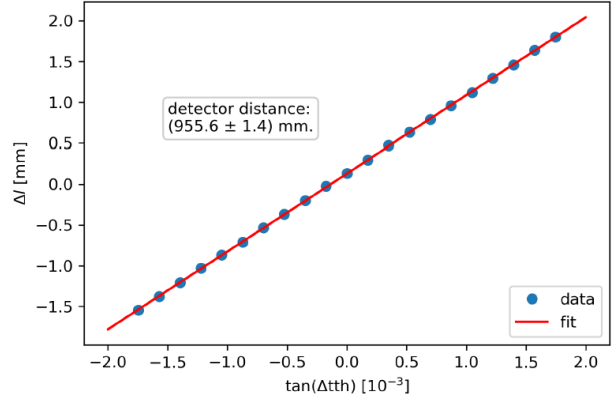

FIG. S3. **Determination of the detector distance.** The detector distance is determined by a fit of a single  $\theta$ - $2\theta$  scan of a sample. The silicon peak is extracted from the detector picture, as described in the main document. Then the change of the peak's pixel position is plotted versus the tan of the change in  $2\theta$  at each step of the incidence angle. The slope of a linear fit yields the detector distance with a value of  $955.6 \pm 1.4$  mm.

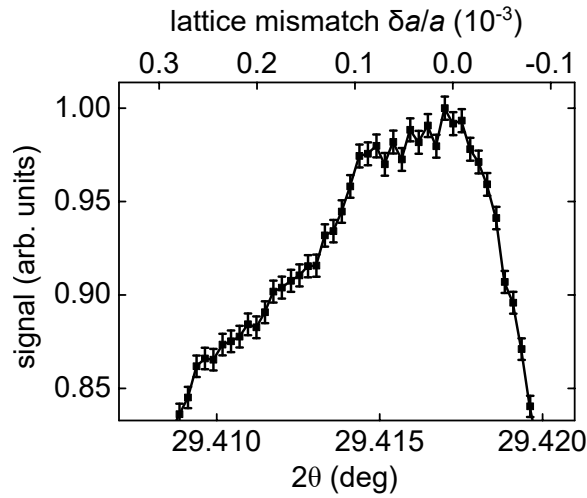

FIG. S4. **Main silicon Bragg peak with error bars.** Radial  $\theta - 2\theta$  scan of the main silicon (400) Bragg peak in the out-of-plane sample direction in the as-prepared state without an electrolyte solution. Error bars denote the uncertainty of the single data point. The ordinate is in linear scale, the abscissa shows angle  $2\theta$  at the bottom and lattice mismatch  $\delta a/a_{\perp}$  with respect to the main silicon peak at the top.

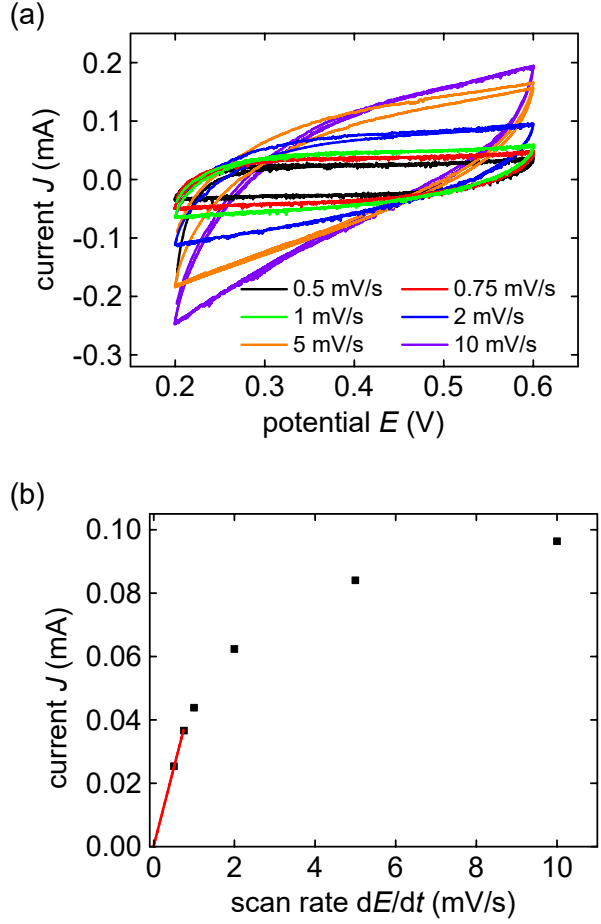

FIG. S5. **Electrochemical characterisation of sample  $S_{\text{trans}}$ .** (a) The graph depicts exemplary cyclic voltammetry measurements of porous silicon polypyrrole hybrid sample  $S_{\text{trans}}$  in  $1 \text{ mol l}^{-1} \text{ HClO}_4$  electrolyte solution in the in situ electrochemical measurement cell. The current  $J$  is plotted against the applied potential  $E$  in the range of  $0.4 - 0.8 \text{ V}$ , measured versus the standard hydrogen potential (SHE). The potential scan rate is increased from  $0.5 \text{ mVs}^{-1}$  to  $10 \text{ mVs}^{-1}$ . (b) The graph depicts values for the porous silicon specific volume specific current  $j$ , averaged in the potential range of  $0.55 - 0.65 \text{ V}$ , plotted against increasing potential scan rates  $dE/dt$  from  $0.5 \text{ mVs}^{-1}$  to  $10 \text{ mVs}^{-1}$ . The red line indicates a linear regression of the first two data points which yields the capacitance  $c_{\text{norm,trans}} = 0.0308 \pm 0.0006 \text{ Fmm}^{-3}$  as the slope.

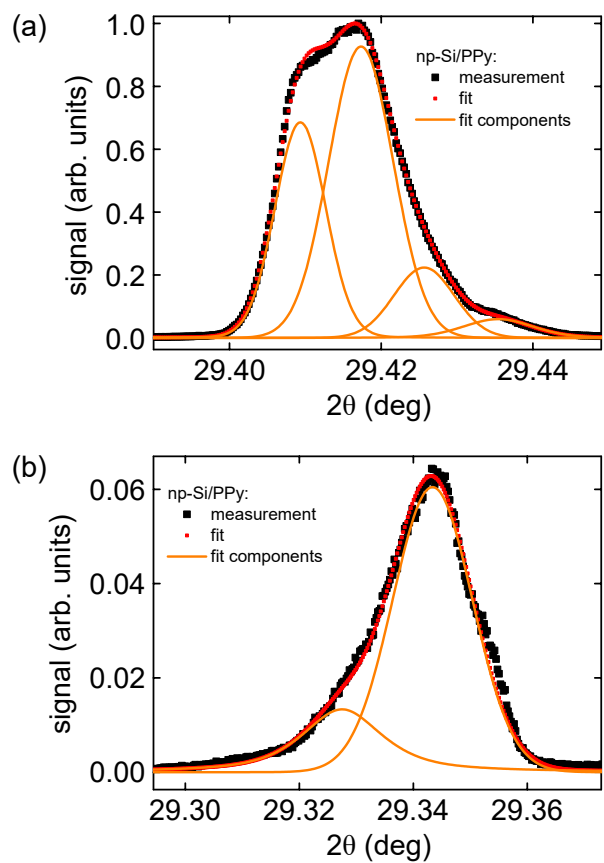

FIG. S6. **Result of the fitting process of bulk silicon and porous silicon peak.** The graph depicts the (400) Bragg peaks of the bulk silicon layer (a) and the porous silicon layer (b) in the out of plane direction of the as prepared sample along with the respective pseudo-Voigt fit functions discussed in the paper.

- 
- [1] J. Schultze and K. Jung, Regular nanostructured systems formed electrochemically: Deposition of electroactive polybithiophene into porous silicon, *Electrochimica acta* **40**, 1369 (1995).
